# Supplementary material for: First-principles photoemission spectroscopy of DNA and RNA nucleobases from Koopmans-compliant functionals
Source: arXiv:1606.03227 source file (2016-06-10)
Supplement: Supplementary file 1 [file SI_main.pdf]

# Supporting Information for :
# "First-principles photoemission spectroscopy of DNA and RNA nucleobases from Koopmans-compliant functionals"

Ngoc Linh Nguyen,[1,*] Giovanni Borghi,[1,2] Andrea Ferretti,[2] and Nicola Marzari[1]

[1] *Theory and Simulations of Materials (THEOS), and National Centre for Computational Design and Discovery of Novel Materials (MARVEL), École Polytechnique Fédérale de Lausanne, 1015 Lausanne, Switzerland*

[2] *Centro S3, CNR–Istituto Nanoscienze, 41125 Modena, Italy*

[*] linh.nguyen@epfl.ch

[1] Clowney, L.; Jain, S. C.; Srinivasan, A. R.; Westbrook, J.; Olson, W. K.; Berman, H. M. *Journal of the American Chemical Society* **1996**, *118*, 509–518.

TABLE S1. Bond lengths and angles between atoms in the adenine molecule computed using PBE, PZ, KIPZ, and PBE0. Experimental values are also reported[1].

| | PBE | PZ | KIPZ | PBE0 | EXP |
|---|---|---|---|---|---|
| $N_1$-$C_2$ | 1.359 | 1.347 | 1.353 | 1.348 | 1.338 |
| $C_2$-$N_3$ | 1.355 | 1.314 | 1.331 | 1.339 | 1.332 |
| $N_3$-$C_4$ | 1.353 | 1.350 | 1.353 | 1.344 | 1.342 |
| $C_4$-$C_5$ | 1.408 | 1.367 | 1.385 | 1.394 | 1.382 |
| $C_5$-$C_6$ | 1.417 | 1.418 | 1.419 | 1.410 | 1.409 |
| $C_6$-$N_1$ | 1.361 | 1.324 | 1.340 | 1.349 | 1.349 |
| $C_5$-$N_7$ | 1.401 | 1.389 | 1.395 | 1.394 | 1.385 |
| $N_7$-$C_8$ | 1.329 | 1.304 | 1.315 | 1.315 | 1.312 |
| $C_8$-$N_9$ | 1.395 | 1.372 | 1.385 | 1.382 | 1.367 |
| $N_9$-$C_4$ | 1.393 | 1.378 | 1.385 | 1.382 | 1.376 |
| $C_6$-$N_6$ | 1.366 | 1.339 | 1.351 | 1.356 | 1.337 |
| C6-N1-C2 | 118.019 | 118.706 | 118.336 | 118.103 | 118.800 |
| N1-C2-N3 | 128.987 | 128.323 | 128.634 | 128.749 | 129.000 |
| C2-N3-C4 | 110.821 | 111.361 | 111.179 | 111.211 | 110.800 |
| N3-C4-C5 | 127.012 | 127.162 | 127.035 | 126.919 | 126.900 |
| C4-C5-C6 | 116.204 | 115.493 | 115.777 | 115.944 | 116.900 |
| C5-C6-N1 | 118.956 | 118.955 | 119.038 | 119.073 | 117.600 |
| C4-C5-N7 | 111.567 | 111.546 | 111.471 | 111.335 | 110.700 |
| C5-N7-C8 | 103.891 | 103.427 | 103.655 | 103.921 | 103.900 |
| N7-C8-N9 | 113.201 | 113.882 | 113.589 | 113.315 | 113.800 |
| C8-N9-C4 | 106.738 | 105.768 | 106.147 | 106.680 | 105.900 |
| N9-C4-C5 | 104.603 | 105.377 | 105.138 | 104.749 | 105.700 |
| N3-C4-N9 | 128.385 | 127.462 | 127.826 | 128.332 | 127.400 |
| C6-C5-N7 | 132.229 | 132.961 | 132.752 | 132.721 | 132.300 |
| N1-C6-N6 | 118.884 | 119.834 | 119.249 | 118.687 | 119.000 |
| C5-C6-N6 | 122.159 | 121.210 | 121.713 | 122.239 | 123.400 |

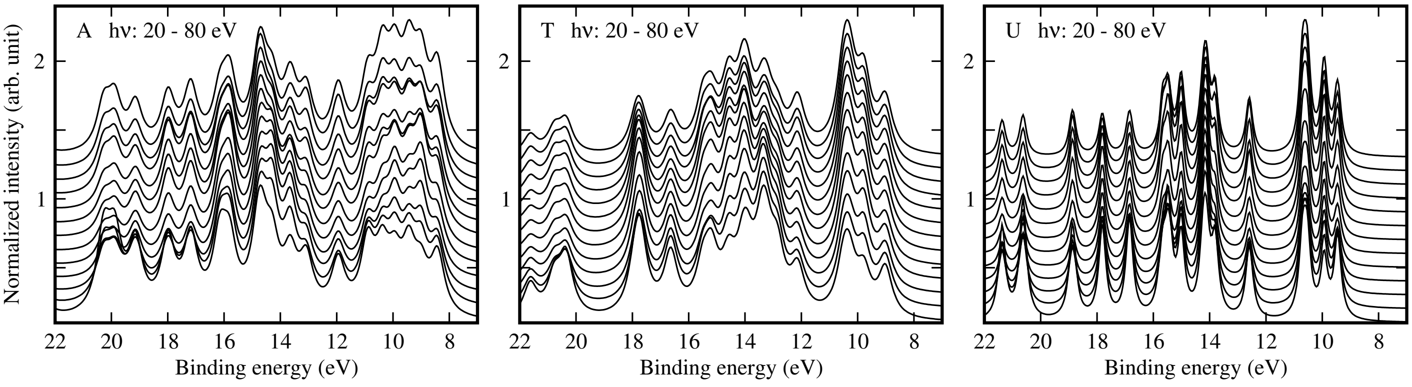


FIG. S1. UPS spectra for adenine, thymine, and uracil computed at different incoming photon energies. The photon energies range between 20 and 80 eV (from bottom to top) with energy steps of 5 eV.

TABLE S2. Bond lengths and angles between the atoms in the thymine molecule computed using PBE, PZ, KIPZ, and PBE0. Experimental values are also reported[1].

| | PBE | PZ | KIPZ | PBE0 | EXP |
|---|---|---|---|---|---|
| N1-C2 | 1.404 | 1.373 | 1.388 | 1.388 | 1.376 |
| C2-N3 | 1.398 | 1.379 | 1.388 | 1.386 | 1.373 |
| N3-C4 | 1.424 | 1.389 | 1.405 | 1.407 | 1.382 |
| C4-C5 | 1.470 | 1.461 | 1.467 | 1.464 | 1.445 |
| C5-C6 | 1.363 | 1.343 | 1.351 | 1.349 | 1.339 |
| C6-N1 | 1.391 | 1.382 | 1.387 | 1.383 | 1.378 |
| C2-O2 | 1.246 | 1.207 | 1.225 | 1.231 | 1.220 |
| C4-O4 | 1.250 | 1.217 | 1.232 | 1.235 | 1.228 |
| C5-C7 | 1.506 | 1.499 | 1.503 | 1.499 | 1.496 |
| N1-C2-O2 | 123.148 | 123.584 | 123.313 | 123.033 | 123.100 |
| N1-C2-N3 | 112.559 | 113.029 | 113.018 | 113.033 | 114.600 |
| O2-C2-N3 | 124.293 | 123.387 | 123.669 | 123.933 | 122.300 |
| C2-N1-C6 | 123.759 | 123.571 | 123.670 | 123.545 | 121.300 |
| C2-N3-C4 | 127.788 | 127.643 | 127.364 | 127.499 | 127.200 |
| N3-C4-O4 | 119.961 | 120.415 | 119.806 | 120.007 | 119.900 |
| N3-C4-C5 | 114.850 | 115.408 | 115.413 | 115.084 | 115.200 |
| O4-C4-C5 | 125.189 | 124.176 | 124.781 | 124.909 | 124.900 |
| C4-C5-C7 | 118.138 | 118.977 | 118.477 | 117.990 | 119.000 |
| C4-C5-C6 | 118.358 | 117.563 | 117.861 | 118.090 | 118.000 |
| C7-C5-C6 | 123.504 | 123.460 | 123.662 | 123.920 | 122.900 |
| N1-C6-C5 | 122.685 | 122.747 | 122.669 | 122.748 | 123.700 |

TABLE S3. Bond lengths and angles between the atoms in the uracil molecule computed using PBE, PZ, KIPZ, and PBE0. Experimental values are also reported[1].

| | PBE | PZ | KIPZ | PBE0 | EXP |
|---|---|---|---|---|---|
| N1-C2 | 1.411 | 1.377 | 1.391 | 1.393 | 1.381 |
| C2-N3 | 1.398 | 1.377 | 1.387 | 1.384 | 1.374 |
| N3-C4 | 1.431 | 1.394 | 1.408 | 1.411 | 1.382 |
| C4-C5 | 1.462 | 1.454 | 1.459 | 1.456 | 1.430 |
| C5-C6 | 1.360 | 1.341 | 1.349 | 1.347 | 1.338 |
| C6-N1 | 1.386 | 1.377 | 1.382 | 1.378 | 1.375 |
| C2-O2 | 1.236 | 1.209 | 1.224 | 1.230 | 1.219 |
| C4-O4 | 1.240 | 1.216 | 1.229 | 1.233 | 1.232 |
| C6-N1-C2 | 123.627 | 123.608 | 123.550 | 123.350 | 121.300 |
| N1-C2-N3 | 112.755 | 113.691 | 113.363 | 113.334 | 114.800 |
| C2-N3-C4 | 127.918 | 126.933 | 127.339 | 127.566 | 127.000 |
| N3-C4-C5 | 113.618 | 115.024 | 114.449 | 113.999 | 114.700 |
| C4-C5-C6 | 120.214 | 118.963 | 119.453 | 119.790 | 119.200 |
| C5-C6-N1 | 121.867 | 121.781 | 121.845 | 121.961 | 122.800 |
| N1-C2-O2 | 122.634 | 122.589 | 122.681 | 122.576 | 123.200 |
| N3-C2-O2 | 124.610 | 123.720 | 123.956 | 124.089 | 122.000 |
| N3-C4-O4 | 119.896 | 119.829 | 119.839 | 119.926 | 119.800 |
| C5-C4-O4 | 126.486 | 125.147 | 125.712 | 126.075 | 125.400 |

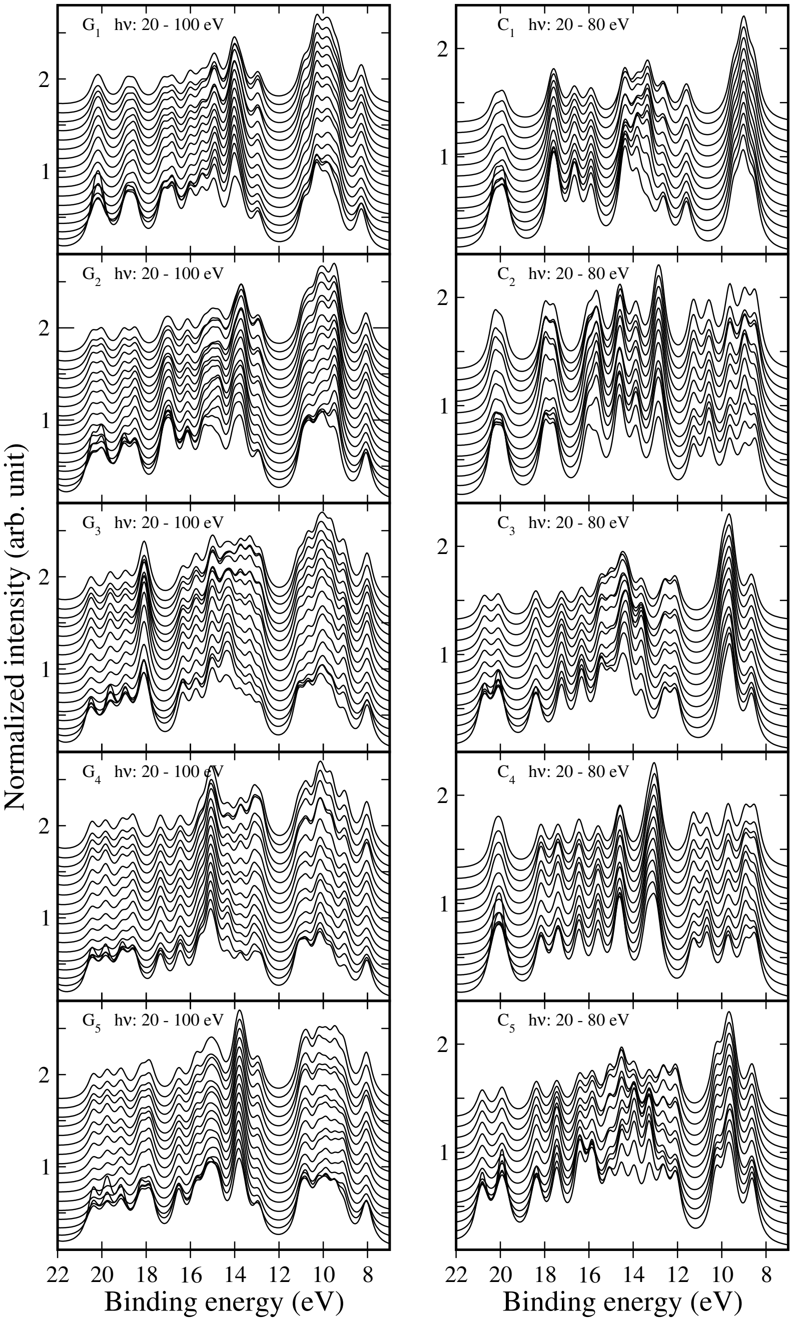


FIG. S2. UPS spectra for the five guanine and cytosine tautomers computed at different incoming photon energies. For cytosine the photon energies range between 20 and 80 eV (from bottom to top), while for guanine they are between 20 and 100 eV (from bottom to top), with energy steps of 5 eV.

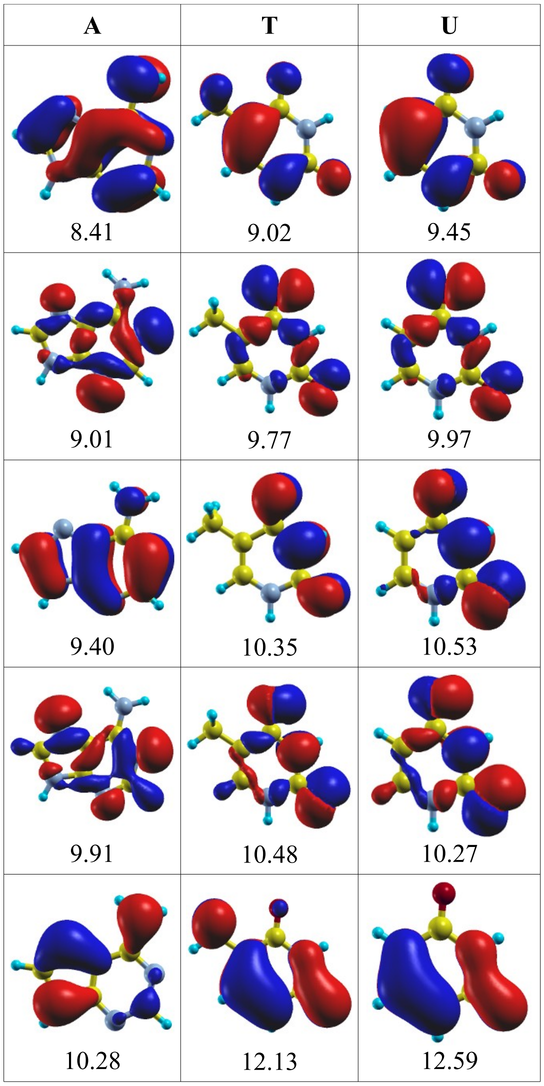


FIG. S3. Iso-surface plots for the highest occupied orbitals of adenine, thymine, and uracil molecules. Binding energies with respect to vacuum computed with KIPZ are shown below each orbital (eV units). Different colors refer to the sign of the wave functions.

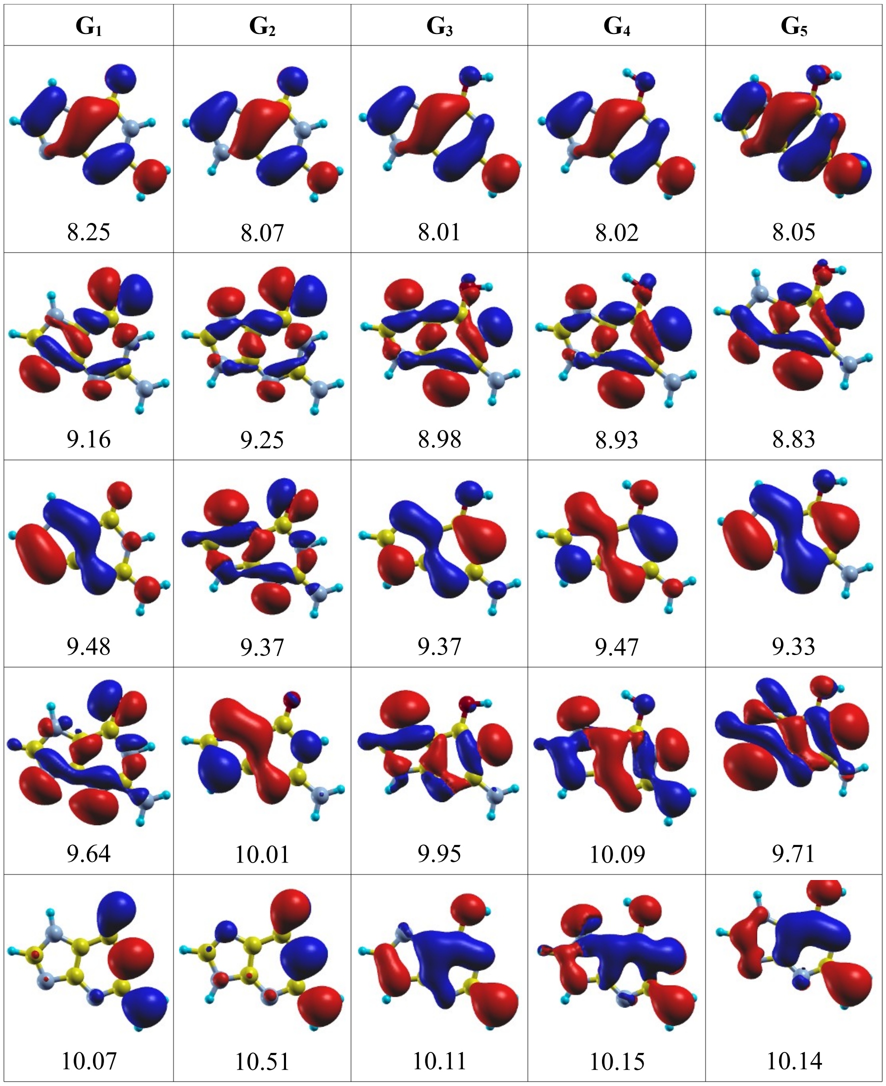


FIG. S4. Iso-surface plots for the highest occupied orbitals of guanine tautomers. Binding energies with respect to vacuum computed with KIPZ are shown below each orbital (eV units). Different colors refer to the sign of the wave functions.

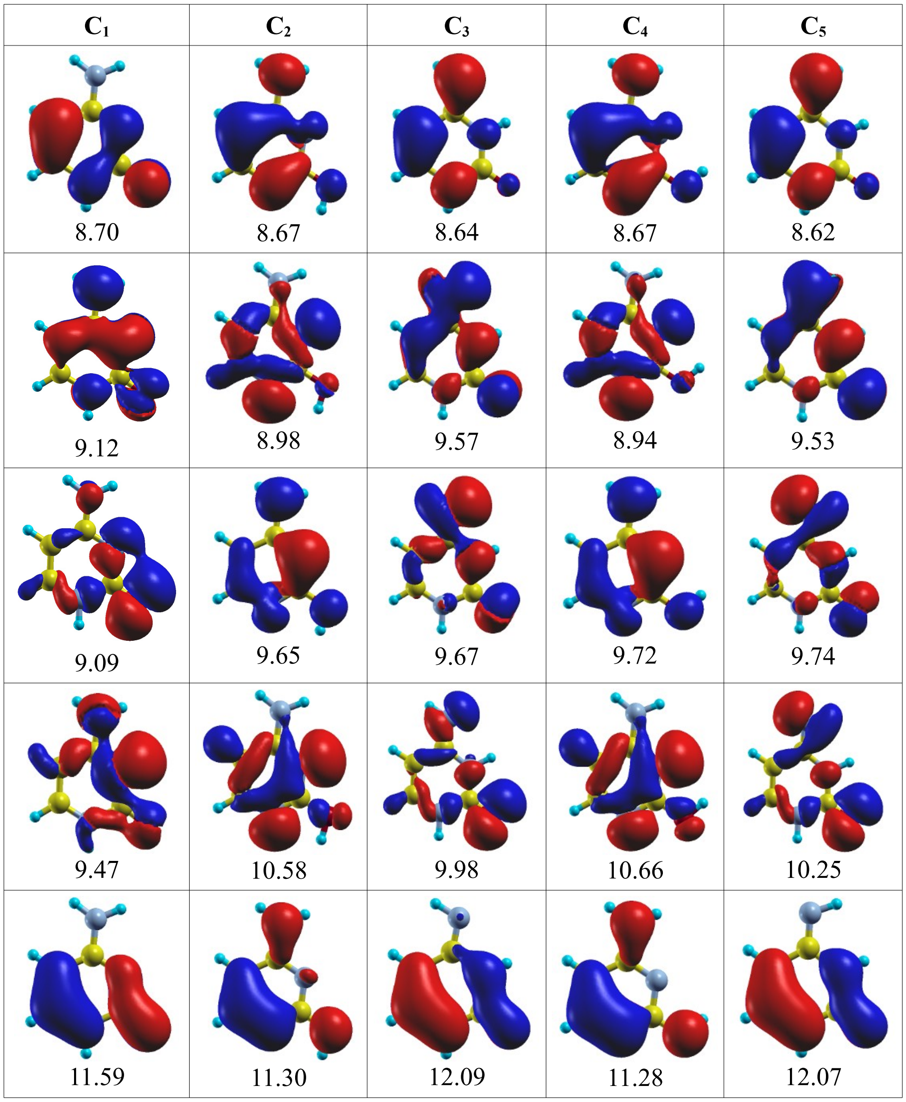


FIG. S5. Iso-surface plots for the highest occupied orbitals of cytosine tautomers. Binding energies with respect to vacuum computed with KIPZ are shown below each orbital (eV units). Different colors refer to the sign of the wave functions.

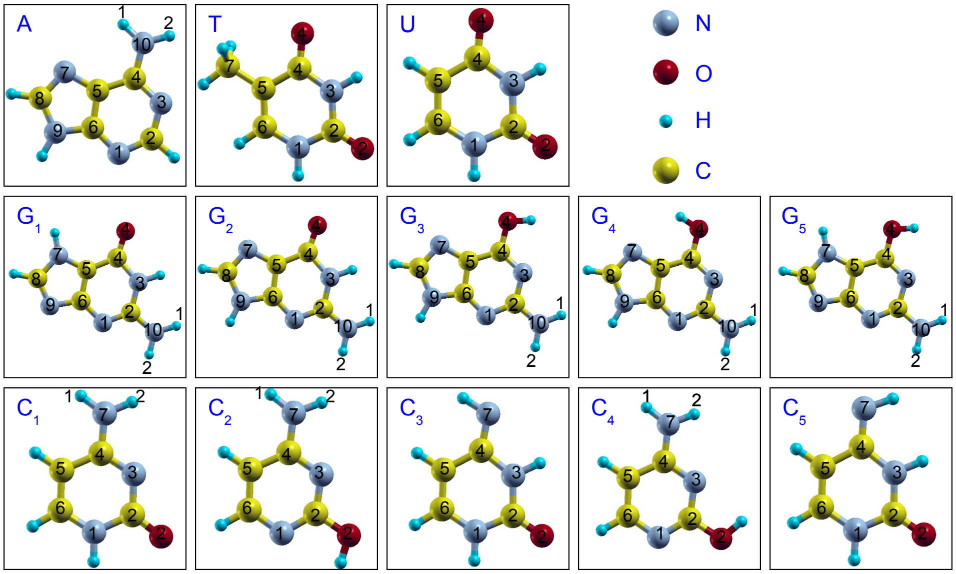


FIG. S6. Structure and indexing of A, T, U, and the five most stable tautomers of G and C, as described in Table IV of the main manuscript and in Table S1, S2, and S3 of this Supporting Information.
